# Supplementary material for: DiTFastAttnV2: Head-wise Attention Compression for Multi-Modality Diffusion Transformers
Source: arXiv:2503.22796 source file (2025-03-28)
Supplement: Supplementary file 1 [file 6_appendix.tex]

\section{Appendix}
